# Supplementary material for: What is SemEval evaluating? A Systematic Analysis of Evaluation Campaigns in NLP
Source: arXiv:2005.14299 ancillary file (2020-05-28)
Supplement: Supplementary file 1 [file appendix_b.pdf]

# What is SemEval evaluating?

## A Systematic Analysis of Evaluation Campaigns in NLP

## Appendix B

| Task ID | Full Name | Citations | Task Type | Task Group | Input | Output | Evaluation Metric | Languages | No of Teams |
|---|---|---|---|---|---|---|---|---|---|
| 2012_01 | 1. English Lexical Simplification[1] | 103 | lexical simplification | OT | word, paragraph, phrase | phrase | kappa index | English | 5 |
| 2012_02 | 2. Measuring Degrees of Relational Similarity[2] | 122 | relational similarity | SEM | word, class label | score | MaxDiff, Spearman Correlation | English | 3 |
| 2012_03 | 3. Spatial Role Labeling[3] | 39 | information extraction | IE | entity, text | entity, attribute, class label, text | recall, F1, precision | English | 1 |
| 2012_04 | 4. Evaluating Chinese Word Similarity[4] | 35 | semantic similarity | SEM | word | score real value | Kendall's $\tau$ | Chinese | 2 |
| 2012_05 | 5. Chinese Semantic Dependency Parsing[5] | 16 | semantic parsing | SEM | sentence | semantic graph | LAS, UAS | Chinese | 5 |
| 2012_06 | 6. Semantic Textual Similarity[6] | 363 | semantic similarity | SEM | sentence | score whole value | Pearson Correlation | English, French | 35 |
| 2012_07 | 7. COPA: Choice Of Plausible Alternatives An evaluation of commonsense causal reasoning[7] | 11 | question answering | QA | sentence | class label | accuracy | English | 1 |
| 2012_08 | 8. Cross-lingual Textual Entailment for Content Synchronization[8] | 34 | machine translation | MT | text | class label | accuracy | English, Spanish, Italian, French, German | 10 |

---

[1] "SemEval-2012 Task 1: English Lexical Simplification - ACL ...." https://www.aclweb.org/anthology/S12-1046. Accessed 28 May. 2020.
[2] "SemEval-2012 Task 2: Measuring Degrees of Relational ...." 7 Jun. 2012, https://www.aclweb.org/anthology/S12-1047.pdf. Accessed 28 May. 2020.
[3] "SemEval-2013 Task 3: Spatial Role Labeling - ACL Anthology." https://www.aclweb.org/anthology/S13-2044. Accessed 28 May. 2020.
[4] "SemEval-2012 Task 4: Evaluating Chinese Word Similarity ...." https://www.aclweb.org/anthology/S12-1049. Accessed 28 May. 2020.
[5] "SemEval-2012 Task 5: Chinese Semantic Dependency Parsing." https://www.aclweb.org/anthology/S12-1050. Accessed 28 May. 2020.
[6] "SemEval-2012 Task 6: A Pilot on Semantic Textual Similarity ...." https://www.aclweb.org/anthology/S12-1051. Accessed 28 May. 2020.
[7] "SemEval-2012 Task 7: Choice of Plausible Alternatives: An ...." https://www.aclweb.org/anthology/S12-1052. Accessed 28 May. 2020.
[8] "Semeval-2012 Task 8: Cross-lingual Textual Entailment for ...." https://www.aclweb.org/anthology/S12-1053. Accessed 28 May. 2020.

| | | | | | | | | | |
|---|---|---|---|---|---|---|---|---|---|
| 2013_01 | 1. TempEval-3 Temporal Annotation[9] | 213 | information extraction | IE | paragraph | paragraph | F1 | English | 9 |
| 2013_02 | 2. Sentiment Analysis in Twitter[10] | 195 | sentiment analysis | SA | word, paragraph | class label | F1 | English | 44 |
| 2013_03 | 3. Spatial Role Labeling[11] | 29 | information extraction | IE | entity, text | entity, class label, text | recall, F1, precision | English | 1 |
| 2013_04 | 4. Free Paraphrases of Noun Compounds[12] | 30 | semantic similarity | SEM | phrase | phrase | ? | English | 3 |
| 2013_05 | 5. Evaluating Phrasal Semantics[13] | 23 | semantic inference | SEM | word, sentence, phrase | ?, class label | accuracy, F1 | English, Italian, French, German | 5 |
| 2013_07 | 7. The Joint Student Response Analysis and 8th Recognizing Textual Entailment Challenge[14] | 76 | semantic inference | SEM | sentence | class label | F1 | English | 9 |
| 2013_08 | 8. Cross-lingual Textual Entailment for Content Synchronization[15] | 10 | semantic inference | SEM | paragraph | class label | accuracy | English, Spanish, Italian, French, German | 6 |
| 2013_09 | 9. Extraction of Drug-Drug Interactions from BioMedical Texts[16] | 170 | information extraction | IE | text | class label, entity | F1 | English | 14 |
| 2013_10 | 10. Cross-lingual Word Sense Disambiguation[17] | 42 | machine translation | MT | ? | ? | precision | English, Italian, French, German, Dutch | 5 |
| 2013_11 | 11. Evaluating Word Sense Induction & Disambiguation within An End-User Application[18] | 48 | question answering | QA | query, paragraph | paragraph | custom evaluation | English | 5 |

[9] "SemEval-2013 Task 1: TempEval-3: Evaluating Time ...." 14 Jun. 2013, https://www.aclweb.org/anthology/S13-2001.pdf. Accessed 28 May. 2020.
[10] "SemEval-2013 Task 2: Sentiment Analysis in Twitter." 14 Jun. 2013, https://www.aclweb.org/anthology/S13-2052.pdf. Accessed 28 May. 2020.
[11] "SemEval-2013 Task 3: Spatial Role Labeling - ACL Anthology." https://www.aclweb.org/anthology/S13-2044. Accessed 28 May. 2020.
[12] "SemEval-2013 Task 4: Free Paraphrases of Noun Compounds." https://www.aclweb.org/anthology/S13-2025. Accessed 28 May. 2020.
[13] "SemEval-2013 Task 5: Evaluating Phrasal Semantics - ACL ...." https://www.aclweb.org/anthology/S13-2007. Accessed 28 May. 2020.
[14] "SemEval-2013 Task 7: The Joint Student Response Analysis ...." https://www.aclweb.org/anthology/S13-2045. Accessed 28 May. 2020.
[15] "Semeval-2013 Task 8: Cross-lingual Textual Entailment ... - ACL." https://www.aclweb.org/anthology/S13-2005. Accessed 28 May. 2020.
[16] "SemEval-2013 Task 9 : Extraction of Drug-Drug Interactions ...." https://www.aclweb.org/anthology/S13-2056. Accessed 28 May. 2020.
[17] "SemEval-2013 Task 10: Cross-lingual Word Sense ... - cs.York." https://www.cs.york.ac.uk/semeval-2013/accepted/25_Paper.pdf. Accessed 28 May. 2020.
[18] "SemEval-2013 Task 11: Word Sense Induction and ...." https://www.aclweb.org/anthology/S13-2035. Accessed 28 May. 2020.

| | | | | | | | | | |
|---|---|---|---|---|---|---|---|---|---|
| 2013_12 | 12. Multilingual Word Sense Disambiguation[19] | 107 | semantic labeling | SEM | text | text | F1 | English, Spanish, Italian, French, German | 3 |
| 2013_13 | 13. Word Sense Induction for Graded and Non-Graded Senses[20] | 49 | word sense disambiguation | OT | text | text | ? | English | 4 |
| 2014_01 | 1. Evaluation of Compositional Distributional Semantic Models on Full Sentences through Semantic Relatedness and Entailment[21] | 374 | semantic similarity | SEM | sentence | score real value, class label | accuracy, Pearson Correlation | English | 21 |
| 2014_02 | 2. Grammar Induction for Spoken Dialogue Systems [22] | 0 | semantic similarity | SEM | phrase | class label | recall, F1, precision | English, Greek | 3 |
| 2014_03 | 3. Cross-Level Semantic Similarity[23] | 42 | semantic similarity | SEM | word, phrase, entity, paragraph, sentence | score real value | Pearson Correlation | English | 19 |
| 2014_04 | 4. Aspect Based Sentiment Analysis[24] | 344 | sentiment analysis | SA | entity, sentence | class label, entity | accuracy, F1 | English | 32 |
| 2014_05 | 5. L2 Writing Assistant[25] | 4 | machine translation | MT | partial sentence, phrase | sentence | accuracy | English, Spanish, French, German, Dutch | 6 |
| 2014_06 | 6. Supervised Semantic Parsing of Spatial Robot Commands[26] | 15 | semantic parsing | SEM | sentence | program | ? | English | 6 |
| 2014_07 | 7. Analysis of Clinical Text[27] | 96 | information extraction | IE | document | entity, phrase | accuracy, F1 | English | 21 |
| 2014_08 | 8. Broad-Coverage Semantic Dependency Parsing[28] | 98 | semantic parsing | SEM | ? | ? | accuracy | English, Czech | 8 |

[19] "SemEval-2013 Task 12: Multilingual Word Sense ...." https://www.aclweb.org/anthology/S13-2040. Accessed 28 May. 2020.
[20] "SemEval-2013 Task 13: Word Sense Induction for Graded and ...." https://www.aclweb.org/anthology/S13-2049. Accessed 28 May. 2020.
[21] "SemEval-2014 Task 1: Evaluation of Compositional ...." 24 Aug. 2014, https://www.aclweb.org/anthology/S14-2001.pdf. Accessed 28 May. 2020.
[22] "Grammar Induction for Spoken Dialogue Systems - ACL ...." https://www.aclweb.org/anthology/S14-2002. Accessed 28 May. 2020.
[23] "SemEval-2014 Task 3: Cross-Level Semantic Similarity - ACL ...." https://www.aclweb.org/anthology/S14-2003. Accessed 28 May. 2020.
[24] "SemEval-2014 Task 4: Aspect Based Sentiment Analysis ...." https://www.aclweb.org/anthology/S14-2004. Accessed 28 May. 2020.
[25] "SemEval 2014 Task 5 - L2 Writing Assistant - ACL Anthology." https://www.aclweb.org/anthology/S14-2005. Accessed 28 May. 2020.
[26] "SemEval-2014 Task 6: Supervised Semantic Parsing of ...." https://www.aclweb.org/anthology/S14-2006. Accessed 28 May. 2020.
[27] "SemEval-2014 Task 7: Analysis of Clinical Text - ACL Anthology." https://www.aclweb.org/anthology/S14-2007. Accessed 28 May. 2020.
[28] "SemEval 2014 Task 8: Broad-Coverage Semantic ... - ACL." https://www.aclweb.org/anthology/S14-2008. Accessed 28 May. 2020.

| | | | | | | | | | |
|---|---|---|---|---|---|---|---|---|---|
| 2014_09 | 9. Sentiment Analysis in Twitter[29] | 3 | sentiment analysis | SA | paragraph, phrase | class label | recall, F1, precision | English | 46 |
| 2014_10 | 10. Multilingual Semantic Textual Similarity[30] | 153 | semantic similarity | SEM | sentence | score whole value | Pearson Correlation | English, Spanish | 9 |
| 2015_01 | Task 1: Paraphrase and Semantic Similarity in Tw[31] itter | 70 | semantic similarity | SEM | sentence | score real value, class label | Pearson Correlation, F1 | English | 19 |
| 2015_02 | Task 2: Semantic Textual Similarity, English, Spanish and Pilot on Interpretability[32] | 161 | semantic similarity | SEM | sentence | score whole value | Pearson Correlation | English, Spanish | 29 |
| 2015_03 | Task 3: Answer Selection in Community Question Answering[33] | 56 | question answering | QA | question, answer | class label | F1 | English, Arabic | 13 |
| 2015_04 | Task 4: TimeLine: Cross-Document Event Ordering[34] | 43 | temporal analysis | OT | document, entity | timeline | F1 | English | 4 |
| 2015_05 | Task 5: QA TempEval[35] | 24 | temporal analysis | OT | document | document | recall | English | 2 |
| 2015_06 | Task 6: Clinical TempEval[36] | 83 | information extraction | IE | paragraph | paragraph | recall, F1, precision | English | 3 |
| 2015_07 | Task 7: Diachronic Text Evaluation[37] | 31 | information extraction | IE | paragraph, KB, phrase | time interval, phrase | accuracy | English | 4 |
| 2015_08 | Task 8: SpaceEval[38] | 21 | information extraction | IE | attribute, paragraph | attribute, class label, paragraph | recall, F1, precision | English | 3 |
| 2015_09 | Task 9: CLIPEval Implicit Polarity of Events[39] | 13 | sentiment analysis | SA | sentence | class label | recall, F1, precision | English | 2 |
| 2015_10 | Task 10: Sentiment Analysis in Twitter[40] | 252 | sentiment analysis | SA | topic, paragraph, phrase | score real value, class label | Kendall's $\tau$ , F1, AvgDiff | English | 41 |
| 2015_11 | Task 11: Sentiment Analysis of Figurative Language in Twitter[41] | 102 | sentiment analysis | SA | paragraph | score whole value | cosine similarity | English | 15 |

[29] "SemEval-2014 Task 9: Sentiment Analysis in Twitter - ACL." 24 Aug. 2014, https://www.aclweb.org/anthology/S14-2009.pdf. Accessed 28 May. 2020.
[30] "SemEval-2014 Task 10: Multilingual Semantic Textual Similarity." https://www.aclweb.org/anthology/S14-2010. Accessed 28 May. 2020.
[31] "SemEval-2015 Task 1: Paraphrase and Semantic Similarity in ...." https://www.aclweb.org/anthology/S15-2001. Accessed 28 May. 2020.
[32] "SemEval-2015 Task 2: Semantic Textual Similarity, English ...." https://www.aclweb.org/anthology/S15-2045. Accessed 28 May. 2020.
[33] "SemEval-2015 Task 3: Answer Selection in Community ...." https://www.aclweb.org/anthology/S15-2047. Accessed 28 May. 2020.
[34] "SemEval-2015 Task 4: TimeLine: Cross-Document Event ...." https://www.aclweb.org/anthology/S15-2132. Accessed 28 May. 2020.
[35] "SemEval-2015 Task 5: QA TempEval - Evaluating Temporal ...." https://www.aclweb.org/anthology/S15-2134. Accessed 28 May. 2020.
[36] "SemEval-2015 Task 6: Clinical TempEval - ACL Anthology." https://www.aclweb.org/anthology/S15-2136. Accessed 28 May. 2020.
[37] "SemEval 2015, Task 7: Diachronic Text Evaluation." https://www.aclweb.org/anthology/S15-2147.pdf. Accessed 28 May. 2020.
[38] "SemEval-2015 Task 8: SpaceEval - ACL Anthology." https://www.aclweb.org/anthology/S15-2149. Accessed 28 May. 2020.
[39] "SemEval-2015 Task 9: CLIPEval Implicit Polarity of Events ...." https://www.aclweb.org/anthology/S15-2077. Accessed 28 May. 2020.
[40] "SemEval-2015 Task 10: Sentiment Analysis in Twitter - ACL ...." https://www.aclweb.org/anthology/S15-2078. Accessed 28 May. 2020.
[41] "SemEval-2015 Task 11: Sentiment Analysis of Figurative ...." http://alt.qcri.org/semeval2015/task11/. Accessed 28 May. 2020.

| | | | | | | | | | |
|---|---|---|---|---|---|---|---|---|---|
| 2015_12 | Task 12: Aspect Based Sentiment Analysis[42] | 214 | sentiment analysis | SA | ?, attribute, entity, sentence | ?, attribute, class label, entity, phrase | ?, F1 | English | 16 |
| 2015_13 | Task 13: Multilingual All-Words Sense Disambiguation and Entity Linking[43] | 85 | entity linking | OT | document | document | recall, F1, precision | English, Spanish, Italian | 9 |
| 2015_14 | Task 14: Analysis of Clinical Text[44] | 53 | information extraction | IE | entity, text | attribute, entity | F*WA, strict F | English | 16 |
| 2015_15 | Task 15: A CPA Dictionary-Entry-Building Task[45] | 2 | semantic parsing | SEM | text, sentence | ?, text, sentence | F1 | English | 5 |
| 2015_17 | Task 17: Taxonomy Extraction Evaluation[46] | 43 | taxonomy extraction | OT | word | word | recall, F1, precision | English | 6 |
| 2015_18 | Task 18: Semantic Dependency Parsing[47] | 0 | semantic parsing | SEM | ? | ? | accuracy | English, Italian, Czech | 6 |
| 2016_01 | Task 1: Semantic Textual Similarity, Monolingual and Cross-Lingual Evaluation[48] | 150 | semantic similarity | SEM | paragraph | score real value | Pearson Correlation | English, Spanish | 43 |
| 2016_02 | Task 2: Interpretable Semantic Textual Similarity[49] | 26 | semantic similarity | SEM | sentence | score whole value | ? | English | 9 |
| 2016_03 | Task 3: Community Question Answering[50] | 123 | semantic similarity | SEM | question, answer | question, answer | MAP | English, Arabic | 18 |
| 2016_04 | Task 4: Sentiment Analysis in Twitter[51] | 436 | sentiment analysis | SA | paragraph, phrase | probability distribution, class label | MAE, Kullback-Leibler Divergence, recall, F1, Earth Mover's Distance | English | 14 |
| 2016_05 | Task 5: Aspect-Based Sentiment Analysis[52] | 465 | sentiment analysis | SA | ?, paragraph, entity, sentence | ?, class label, entity, phrase | accuracy, F1 | English, Spanish, French, Arabic, Dutch, Chinese, | 29 |

42 "SemEval-2015 Task 12: Aspect Based Sentiment Analysis ...." https://www.aclweb.org/anthology/S15-2082/. Accessed 28 May. 2020.
43 "SemEval-2015 Task 13: Multilingual All-Words Sense ... - ACL." https://www.aclweb.org/anthology/S15-2049. Accessed 28 May. 2020.
44 "SemEval-2015 Task 14: Analysis of Clinical Text - ACL ...." https://www.aclweb.org/anthology/S15-2051. Accessed 28 May. 2020.
45 "SemEval-2015 Task 15: A CPA dictionary-entry-building task." https://www.aclweb.org/anthology/S15-2053.pdf. Accessed 28 May. 2020.
46 "SemEval-2015 Task 17: Taxonomy Extraction Evaluation ...." https://www.aclweb.org/anthology/S15-2151. Accessed 28 May. 2020.
47 "SemEval 2015 Task 18: Broad-Coverage Semantic ...." https://www.aclweb.org/anthology/S15-2153. Accessed 28 May. 2020.
48 "SemEval-2016 Task 1: Semantic Textual Similarity ...." https://www.aclweb.org/anthology/S16-1081. Accessed 28 May. 2020.
49 "SemEval-2016 Task 2: Interpretable Semantic Textual Similarity." https://www.aclweb.org/anthology/S16-1082. Accessed 28 May. 2020.
50 "SemEval-2016 Task 3: Community Question Answering - ACL ...." https://www.aclweb.org/anthology/S16-1083. Accessed 28 May. 2020.
51 "SemEval-2016 Task 4: Sentiment Analysis in Twitter - ACL ...." https://www.aclweb.org/anthology/S16-1001. Accessed 28 May. 2020.
52 "SemEval-2016 Task 5: Aspect Based Sentiment Analysis ...." https://www.aclweb.org/anthology/S16-1002. Accessed 28 May. 2020.

| | | | | | | | | | |
|---|---|---|---|---|---|---|---|---|---|
| | | | | | | | | Turkish, Russian | |
| 2016_06 | Task 6: Detecting Stance in Tweets[53] | 209 | sentiment analysis | SA | paragraph, phrase | class label | F1 | English | 28 |
| 2016_07 | Task 7: Determining Sentiment Intensity of English and Arabic Phrases[54] | 39 | sentiment analysis | SA | phrase | score real value | Kendall's $\tau$ | English, Arabic | 5 |
| 2016_08 | Task 8: Meaning Representation Parsing[55] | 28 | semantic parsing | SEM | sentence | semantic graph | Smatch | English | 11 |
| 2016_09 | Task 9: Chinese Semantic Dependency Parsing[56] | 0 | semantic parsing | SEM | KB, sentence | semantic graph | F1 | Chinese | 3 |
| 2016_10 | Task 10: Detecting Minimal Semantic Units and their Meanings[57] | 23 | semantic analysis | SEM | paragraph | entity | F1 | English | 6 |
| 2016_11 | Task 11: Complex Word Identification[58] | 40 | lexical simplification | OT | word, sentence | class label | F1 | English | 21 |
| 2016_12 | Task 12: Clinical TempEval[59] | 79 | information extraction | IE | paragraph | paragraph | recall, F1, precision | English | 14 |
| 2016_13 | Task 13: Taxonomy Extraction Evaluation (TExEval-2)[60] | 54 | taxonomy extraction | OT | word, KB | word, DAG | human judgement, recall, F1, Cumulative F&M, precision | English, Italian, French, Dutch | 5 |
| 2016_14 | Task 14: Semantic Taxonomy Enrichment[61] | 10 | taxonomy enrichment | OT | word, sentence | class label, entity | accuracy, recall | English | 5 |
| 2017_01 | Task 1: Semantic Textual Similarity[62] | 144 | semantic similarity | SEM | sentence | score real value | Pearson Correlation | English, Spanish, Arabic, Turkish | 31 |
| 2017_02 | Task 2: Multi-lingual and Cross-lingual Semantic Word Similarity[63] | 56 | semantic similarity | SEM | word | score real value | Pearson Correlation, Spearman Correlation | English, Spanish, Italian, German, | 17 |

53 "SemEval-2016 Task 6: Detecting Stance in Tweets - ACL ...." https://www.aclweb.org/anthology/S16-1003. Accessed 28 May. 2020.
54 "SemEval-2016 Task 7: Determining Sentiment Intensity ... - ACL." https://www.aclweb.org/anthology/S16-1004. Accessed 28 May. 2020.
55 "SemEval-2016 Task 8: Meaning Representation Parsing ...." https://www.aclweb.org/anthology/S16-1166. Accessed 28 May. 2020.
56 "SemEval-2016 Task 9: Chinese Semantic Dependency Parsing." https://www.aclweb.org/anthology/S16-1167. Accessed 28 May. 2020.
57 "SemEval-2016 Task 10: Detecting Minimal Semantic Units ...." https://www.aclweb.org/anthology/S16-1084. Accessed 28 May. 2020.
58 "SemEval 2016 Task 11: Complex Word Identification - ACL ...." https://www.aclweb.org/anthology/S16-1085. Accessed 28 May. 2020.
59 "SemEval-2017 Task 12: Clinical TempEval - ACL Anthology." https://www.aclweb.org/anthology/S17-2093. Accessed 28 May. 2020.
60 "SemEval-2016 Task 13: Taxonomy Extraction Evaluation ...." https://www.aclweb.org/anthology/S16-1168. Accessed 28 May. 2020.
61 "SemEval-2016 Task 14: Semantic Taxonomy Enrichment ...." https://www.aclweb.org/anthology/S16-1169. Accessed 28 May. 2020.
62 "SemEval-2017 Task 1: Semantic Textual Similarity ...." https://www.aclweb.org/anthology/S17-2001. Accessed 28 May. 2020.
63 "SemEval-2017 Task 2: Multilingual and Cross-lingual Semantic." https://www.aclweb.org/anthology/S17-2002. Accessed 28 May. 2020.

| | | | | | | | | | |
|---|---|---|---|---|---|---|---|---|---|
| | | | | | | | | Persian (Farsi) | |
| 2017_03 | Task 3: Community Question Answering[64] | 106 | semantic similarity | SEM | question, answer | question, answer | MAP | English, Arabic | 23 |
| 2017_04 | Task 4: Sentiment Analysis in Twitter[65] | 307 | sentiment analysis | SA | paragraph, phrase | probability distribution, class label | MAE, Kullback-Leibler Divergence, recall, Earth Mover's Distance | English, Arabic | 48 |
| 2017_05 | Task 5: Fine-Grained Sentiment Analysis on Financial Microblogs and News[66] | 48 | sentiment analysis | SA | paragraph | score real value | cosine similarity | English | 32 |
| 2017_06 | Task 6: #HashtagWars: Learning a Sense of Humor[67] | 15 | sentiment analysis | SA | paragraph | class label, paragraph | accuracy, edit distance | English | 8 |
| 2017_07 | Task 7: Detection and Interpretation of English Puns [68] | 23 | semantic parsing | SEM | word, paragraph | word, class label, entity | standard coverage, recall, F1, precision | English | 10 |
| 2017_08 | Task 8: RumourEval: Determining rumour veracity and support for rumours[69] | 71 | fact checking | IE | tree, paragraph | class label | accuracy | English | 8 |
| 2017_09 | Task 9: Abstract Meaning Representation Parsing and Generation[70] | 15 | semantic parsing | SEM | semantic graph, sentence | semantic graph, sentence | Smatch, human judgement | English | 5 |
| 2017_10 | Task 10: Extracting Keyphrases and Relations from Scientific Publications[71] | 73 | information extraction | IE | word, class label, text | word, class label | recall, F1, precision | English | 26 |
| 2017_11 | Task 11: End-User Development using Natural Language[72] | 4 | machine translation | MT | KB, sentence | program | ? | English, Programing language | 1 |
| 2017_12 | Task 12: Clinical TempEval[73] | 0 | information extraction | IE | paragraph | paragraph | recall, F1, precision | English | 11 |
| 2018_01 | Task 1: Affect in Tweets[74] | 98 | sentiment analysis | SA | entity, paragraph | score real value, class label | Pearson Correlation, Jaccard index | English, Spanish, Arabic | 75 |

---

64 "SemEval-2016 Task 3: Community Question Answering - ACL ...." https://www.aclweb.org/anthology/S16-1083. Accessed 28 May. 2020.
65 "SemEval-2016 Task 4: Sentiment Analysis in Twitter - ACL ...." https://www.aclweb.org/anthology/S16-1001. Accessed 28 May. 2020.
66 "SemEval-2017 Task 5: Fine-Grained Sentiment Analysis on ...." https://www.aclweb.org/anthology/S17-2089/. Accessed 28 May. 2020.
67 "SemEval-2017 Task 6: #HashtagWars: Learning a Sense of ...." https://www.aclweb.org/anthology/S17-2004. Accessed 28 May. 2020.
68 "SemEval-2017 Task 7: Detection and Interpretation of English ...." https://www.aclweb.org/anthology/S17-2005. Accessed 28 May. 2020.
69 "SemEval-2017 Task 8: RumourEval: Determining rumour ...." https://www.aclweb.org/anthology/S17-2006. Accessed 28 May. 2020.
70 "SemEval-2017 Task 9: Abstract Meaning Representation ...." https://www.aclweb.org/anthology/S17-2090. Accessed 28 May. 2020.
71 "SemEval 2017 Task 10: ScienceIE - Extracting Keyphrases ...." https://www.aclweb.org/anthology/S17-2091. Accessed 28 May. 2020.
72 "End-User Development using Natural Language - ACL ...." https://www.aclweb.org/anthology/S17-2092. Accessed 28 May. 2020.
73 "SemEval-2017 Task 12: Clinical TempEval - ACL Anthology." https://www.aclweb.org/anthology/S17-2093. Accessed 28 May. 2020.
74 "SemEval-2018 Task 1: Affect in Tweets - ACL Anthology." https://www.aclweb.org/anthology/S18-1001. Accessed 28 May. 2020.

| | | | | | | | | | |
|---|---|---|---|---|---|---|---|---|---|
| 2018_02 | Task 2: Multilingual Emoji Prediction[75] | 20 | sentiment analysis | SA | paragraph | class label | accuracy, recall, F1, precision | English, Spanish | 49 |
| 2018_03 | Task 3: Irony Detection in English Tweets[76] | 43 | sentiment analysis | SA | paragraph | class label | F1 | English | 43 |
| 2018_04 | Task 4: Character Identification on Multiparty Dialogues[77] | 2 | entity linking | OT | word, text | entity | accuracy, F1 | English | 4 |
| 2018_05 | Task 5: Counting Events and Participants within Highly Ambiguous Data covering a very long tail[78] | 0 | question answering | QA | document, question | number, document | ? | English | 4 |
| 2018_06 | Task 6: Parsing Time Normalizations[79] | 3 | information extraction | IE | text | ?, entity | recall, F1, precision | English | 1 |
| 2018_07 | Task 7: Semantic Relation Extraction and Classification in Scientific Papers[80] | 26 | semantic parsing | SEM | entity, paragraph | class label, entity | F1 | English | 32 |
| 2018_08 | Task 8: Semantic Extraction from CybersecUrity REports using Natural Language Processing (SecureNLP)[81] | 3 | information extraction | IE | sentence | word, attribute, class label | F1 | English | 9 |
| 2018_09 | Task 9: Hypernym Discovery[82] | 13 | hypernym discovery | OT | text, phrase | phrase | MAP | English, Spanish, Italian | 11 |
| 2018_10 | Task 10: Capturing Discriminative Attributes[83] | 5 | semantic difference | SEM | word | class label | F1 | English | 21 |
| 2018_11 | Task 11: Machine Comprehension using Commonsense Knowledge[84] | 33 | question answering | QA | document, question | answer | accuracy | English | 11 |
| 2018_12 | Task 12: Argument Reasoning Comprehension Task[85] | 7 | argument reasoning | IE | paragraph | class label | accuracy | English | 22 |
| 2019_01 | Task 1: Cross-lingual Semantic Parsing with UCCA[86] | 3 | semantic parsing | SEM | semantic graph | ? | ? | English, French, German | 8 |

[75] "SemEval 2018 Task 2: Multilingual Emoji Prediction - ACL ...." https://www.aclweb.org/anthology/S18-1003. Accessed 28 May. 2020.
[76] "SemEval-2018 Task 3: Irony Detection in English Tweets ...." https://www.aclweb.org/anthology/S18-1005. Accessed 28 May. 2020.
[77] "SemEval 2018 Task 4: Character Identification on Multiparty ...." https://www.aclweb.org/anthology/S18-1007. Accessed 28 May. 2020.
[78] "SemEval-2018 Task 5: Counting Events and Participants in ...." 5 Jun. 2018, https://www.aclweb.org/anthology/S18-1009.pdf. Accessed 28 May. 2020.
[79] "SemEval 2018 Task 6: Parsing Time Normalizations - ACL ...." https://www.aclweb.org/anthology/S18-1011. Accessed 28 May. 2020.
[80] "SemEval-2018 Task 7: Semantic Relation Extraction and ...." https://www.aclweb.org/anthology/S18-1111. Accessed 28 May. 2020.
[81] "SemEval-2018 Task 8: Semantic Extraction from ... - ACL." https://www.aclweb.org/anthology/S18-1113. Accessed 28 May. 2020.
[82] "SemEval-2018 Task 9: Hypernym Discovery - ACL Anthology." https://www.aclweb.org/anthology/S18-1115. Accessed 28 May. 2020.
[83] "SemEval-2018 Task 10: Capturing Discriminative Attributes ...." https://www.aclweb.org/anthology/S18-1117. Accessed 28 May. 2020.
[84] "SemEval-2018 Task 11: Machine Comprehension Using - ACL." https://www.aclweb.org/anthology/S18-1119. Accessed 28 May. 2020.
[85] "SemEval-2018 Task 12: The Argument Reasoning ... - ACL." https://www.aclweb.org/anthology/S18-1121. Accessed 28 May. 2020.
[86] "SemEval-2019 Task 1: Cross-lingual Semantic Parsing with ...." https://www.aclweb.org/anthology/S19-2001. Accessed 28 May. 2020.

| | | | | | | | | | |
|---|---|---|---|---|---|---|---|---|---|
| 2019_02 | Task 2: Unsupervised Lexical Semantic Frame Induction[87] | 1 | semantic labeling | SEM | syntactic labeled sentence | entity | BCUBED F-SCORE | English | 13 |
| 2019_03 | Task 3: EmoContext: Contextual Emotion Detection in Text[88] | 11 | sentiment analysis | SA | sentence | class label | recall, F1, precision | English | 311 |
| 2019_04 | Task 4: Hyperpartisan News Detection[89] | 5 | sentiment analysis | SA | text | class label | accuracy | English | 42 |
| 2019_05 | Task 5: HatEval: Multilingual Detection of Hate Speech Against Immigrants and Women in Twitter[90] | 15 | sentiment analysis | SA | paragraph | class label | F1, Exact Match Ratio | English, Spanish | 74 |
| 2019_06 | Task 6: OffensEval: Identifying and Categorizing Offensive Language in Social Media[91] | 13 | sentiment analysis | SA | paragraph | class label | F1 | English | 115 |
| 2019_07 | Task 7: RumourEval 2019: Determining Rumour Veracity and Support for Rumours[92] | 7 | fact checking | IE | paragraph | score real value, class label | RMSE, F1 | English | 22 |
| 2019_08 | Task 8: Fact Checking in Community Question Answering Forums[93] | 4 | fact checking | IE | question, answer | class label | accuracy | English | 17 |
| 2019_09 | Task 9: Suggestion Mining from Online Reviews and Forums[94] | 3 | information extraction | IE | sentence | class label | F1 | English | 33 |
| 2019_10 | Task 10: Math Question Answering[95] | 0 | question answering | QA | question | answer | accuracy | English | 3 |
| 2019_12 | Task 12: Toponym Resolution in Scientific Papers[96] | 2 | entity linking | OT | text, phrase | entity, phrase | recall, F1, precision | English | 8 |

87 "SemEval-2019 Task 2: Unsupervised Lexical Frame Induction ...." https://www.aclweb.org/anthology/S19-2003. Accessed 28 May. 2020.
88 "SemEval-2019 Task 3: EmoContext Contextual Emotion ...." https://www.aclweb.org/anthology/S19-2005. Accessed 28 May. 2020.
89 "SemEval-2019 Task 4: Hyperpartisan News Detection - ACL ...." https://www.aclweb.org/anthology/S19-2145. Accessed 28 May. 2020.
90 "LT3 at SemEval-2019 Task 5: Multilingual Detection of Hate ...." https://www.aclweb.org/anthology/S19-2077. Accessed 28 May. 2020.
91 "SemEval-2019 Task 6: Identifying and Categorizing Offensive ...." https://www.aclweb.org/anthology/S19-2010. Accessed 28 May. 2020.
92 "SemEval-2019 Task 7: RumourEval, Determining Rumour ...." https://www.aclweb.org/anthology/S19-2147. Accessed 28 May. 2020.
93 "SemEval-2019 Task 8: Fact Checking in Community Question ...." https://www.aclweb.org/anthology/S19-2149. Accessed 28 May. 2020.
94 "SemEval-2019 Task 9: Suggestion Mining from Online ...." https://www.aclweb.org/anthology/S19-2151. Accessed 28 May. 2020.
95 "SemEval-2019 Task 10: Math Question Answering - ACL ...." https://www.aclweb.org/anthology/S19-2153. Accessed 28 May. 2020.
96 "SemEval-2019 Task 12: Toponym Resolution in Scientific ...." https://www.aclweb.org/anthology/S19-2155. Accessed 28 May. 2020.
